# Supplementary material for: Designing Computational Tools for Exploring Causal Relationships in Qualitative Data
Source: arXiv:2602.06506 source file (2026-02-06)
Supplement: Supplementary file 1 [file appendix_discard.tex]

\section{Appendix}

\subsection{Technical Details}
\label{app:prompt}

\subsubsection{Indicator Extraction}

Table \ref{tab:indicator_prompt} shows the prompt used for the automatic indicator extraction process described in Section \ref{sec:indicator}.

\begin{table}[h]
\centering
\caption{Prompt for Indicator Extraction}
\label{tab:indicator_prompt}
\begin{tabular}{|p{0.9\textwidth}|}
\hline
\textbf{[Instruction]} \\
Extract meaningful indicators from the provided sentence, which is taken from qualitative data. In grounded theory, an indicator refers to a word, phrase, or sentence, or a series of words, phrases, or sentences, in the materials being analyzed. \\
% \hline
\\

\textbf{[Example]} \\
- Research Overview: "\textit{This study explores emotional responses and conflict resolution strategies in interpersonal relationships, particularly focusing on how individuals manage anger and attempt to mediate tense situations.}"\\
- Sentence: "\textit{No, I would not feel angry, I would feel concerned and try to talk to them to calm them down. It is out of the ordinary behaviour for them, I do not like seeing people angry or arguments so I would try and defuse the situation.}" \\
\\
\textbf{Output:} \\
\begin{verbatim}
{
  "indicators": [
    "I would not feel angry",
    "I would feel concerned", 
    "try to talk to them to calm them down",
    "It is out of the ordinary behaviour for them",
    "I do not like seeing people angry or arguments",
    "I would try and defuse the situation"
  ]
}
\end{verbatim} \\
% \hline
\\

\textbf{[Output Format]} \\
Return the extracted indicators in JSON format as a simple list: \\
\begin{verbatim}
{
  "indicators": [
    "indicator1",
    "indicator2", 
    "indicator3",
    ...
  ]
}
\end{verbatim} \\
% \hline
\\

\textbf{[Input]} \\
- Research Overview: \texttt{(The research context and objectives)}\\
- Sentence: \texttt{(The specific sentence to be extracted)} \\
\hline
\end{tabular}
\end{table}

\subsubsection{Concept Mapping}

Table \ref{tab:construct_mapping} shows the prompt used for automatically assigning concepts to unmapped indicators after theoretical saturation is reached, as described in Section \ref{sec:concept}.

\begin{table}[h]
\centering
\caption{Prompt for Concept Mapping}
\label{tab:construct_mapping}
\begin{tabular}{|p{0.9\textwidth}|}
\hline
\textbf{[Instruction]} \\
Your task is to assign the most appropriate concept to a given indicator (in grounded theory, an indicator refers to a word, phrase, or sentence, or a series of words, phrases, or sentences, in the materials being analyzed). \\
\\
You will be provided with: \\
1. An indicator extracted from a paragraph \\
2. The complete sentence from which the indicator was extracted \\
3. A list of concepts with their definitions and references \\
\\
If you find that none of the concepts seem appropriate, select the one that is the best fit. \\
\\
Answer the following question based on the indicator, sentence, and concepts given to you: \\
\texttt{Which concept best describes the indicator within the context of the sentence?} (Select exactly one option) \\
a. concept1 \\
b. concept2 \\
c. concept3 \\
d. ... \\
% \hline
\\

\textbf{[Output Format]} \\
Please output your choice as a single letter: \\
label: [a/b/c] \\
\\
\textbf{[Input]}\\
- Indicator: \texttt{(The specific indicator to be mapped)} \\
- Sentence: \texttt{(The complete sentence from which the indicator was extracted)} \\
- Concepts:
% \hline
% % \\
% \textbf{[Sentence]} \\
% \texttt{(The complete sentence from which the indicator was extracted)} \\
% % \hline
% \\
% \textbf{[Concepts]} \\
\\
\quad a. concept1: definition1 \\
\quad References: example1a, example1b, example1c \\
\\
\quad b. concept2: definition2 \\
\quad References: example2a, example2b, example2c \\
\\
\quad c. concept3: definition3 \\
\quad References: example3a, example3b, example3c \\
\\
\quad d. ... \\
% \hline
\\
\hline
\end{tabular}
\end{table}

\subsubsection{Causal Relationship Extraction}

Table \ref{tab:causal_relation} shows the prompt used for automated causal inference, which determines the existence and direction of causal relationships between indicator pairs as described in Section \ref{sec:causal}.

\begin{table}[h]
\centering
\caption{Prompt for Causal Relationship Extraction}
\label{tab:causal_relation}
\begin{tabular}{|p{0.9\textwidth}|}

\hline
\textbf{[Instruction]} \\
Analyze the given sentence and the two identified indicators with their concepts. Determine if there is a meaningful causal relationship between these indicators based on the text evidence. A causal relationship exists when one indicator (cause) leads to another indicator (effect). \\
\\
\textbf{IMPORTANT:} \\
1. Consider both explicit causal markers (like "because," "therefore," "since," "as a result") AND implicit causal relationships. While many causal relationships are explicitly indicated, others might be inferred from the meaning and context of the sentence. Both types are equally valid for this task. \\
2. Pay careful attention to the direction of causation: determine which indicator leads to the other, not the reverse. \\
% \hline

\\
You will be provided with: \\
1. Sentence: The complete sentence from qualitative data being analyzed \\
2. Indicator 1: The first indicator with its concept type in parentheses \\
3. Indicator 2: The second indicator with its concept type in parentheses \\
% \hline

\\
% \textbf{[Task]} \\
Answer the following question based on the indicators and sentence given to you: \\
\texttt{Which of the following statements is true?} (Select exactly one option)
\\
% \textbf{Options:} \\
a. Indicator 1 causes Indicator 2 \\
b. Indicator 2 causes Indicator 1 \\
c. Indicator 1 and Indicator 2 are not directly causally related \\
% \hline

\\
\textbf{[Output Format]} \\
Please output your choice as a single letter: \\
label: [a/b/c] \\

\\
\textbf{[Input]} \\
- Sentence: \texttt{(The complete sentence from qualitative data being analyzed)} \\
- Indicator 1: \texttt{(The first indicator with its concept type in parentheses)} \\
- Indicator 2: \texttt{(The second indicator with its concept type in parentheses)} \\
\hline
\end{tabular}
\end{table}

\subsubsection{Indicator Merging}
\label{app:merge}

We performed indicator merging to handle variations in phrasing and consolidate semantically similar indicators following \textit{entity resolution} approaches before causal relationship extraction \cite{causal_text_meng_2025, entity_resolution_peeters_2023}.
For each indicator, we first identified the 10 most semantically similar indicators using word embeddings. 
We then filtered these candidates to retain only those assigned to the same concept. 
For each filtered pair, we prompted the LLM (Table \ref{tab:indicator_merging}) with the original indicators, their shared concept, and source sentences to determine whether the indicators should be merged based on semantic equivalence.

\begin{table}[h]
\centering
\caption{Prompt for Indicator Merging}
\label{tab:indicator_merging}
\begin{tabular}{|p{0.9\textwidth}|}
\hline
\textbf{[Instruction]} \\
Determine if two indicators represent the same real-world indicators (in grounded theory, an indicator refers to a word, phrase, or sentence, or a series of words, phrases, or sentences, in the materials being analyzed) or refer to functionally identical semantic meanings despite different surface forms, based on their concept and the original sentences from which they were extracted. Indicators should ONLY be merged if they are equivalent, not merely related or similar concepts. For merging to be appropriate, the indicators need to be interchangeable in their respective contexts without changing the meaning. \\
\\
You will be provided with: \\
1. Concept: The shared concept assigned to both indicators \\
2. Indicator 1: The first indicator to be compared \\
3. Sentence 1: The sentence from which Indicator 1 was extracted \\
4. Indicator 2: The second indicator to be compared \\
5. Sentence 2: The sentence from which Indicator 2 was extracted \\
\\
Answer the following question based on the indicators and sentences given to you: \\
\texttt{Should these two indicators be merged?} (Select exactly one option) \\
a. Merge \\
b. Do not merge \\
\\
\textbf{[Output Format]} \\
Please output your choice as a single letter: \\
label: [a/b] \\
\\
\textbf{[Input]} \\
- Concept: \texttt{(The shared concept assigned to both indicators)} \\
- Indicator 1: \texttt{(The first indicator to be compared)} \\
- Sentence 1: \texttt{(The sentence from which Indicator 1 was extracted)} \\
- Indicator 2: \texttt{(The second indicator to be compared)} \\
- Sentence 2: \texttt{(The sentence from which Indicator 2 was extracted)} \\
\hline
\end{tabular}
\end{table}
